# Supplementary material for: Coherent phonon transport and minimum of thermal conductivity in LaMnO$_3$/SrMnO$_3$ superlattices
Source: arXiv:2108.05860 source file (2021-08-12)
Supplement: Supplementary file 1 [file supplement.tex]

\appendix\section{\label{sup}Supplementary Material}

\appendix\subsection{\label{sup:samples}Sample characterization}

The LSMO films and LMOn/SMOn superlattice (SL) samples were epitaxially grown on terminated SrTiO3 (100) substrates by means of metalorganic aerosol deposition technique (MAD) analogously to Ref. \cite{Keunecke2020}. The substrate is heated up to \SI{900}{\celsius} via a resistive heater under atmospheric pressure with an oxygen partial pressure of $p_{O_{2}} \approx \SI{0.2}{bar}$. Metalorganic precursors are dissolved in dimethylformamide (DMF) and sprayed through a nozzle onto the sample using dry compressed air and a syringe system. The precusor solution exhibits an empirically determined ratio of La(III)-, Sr(II)-, Mn(II)acetylacetonate (acac) for the LSMO growth. For the SL two precursor solutions were prepared for the LMO and SMO sublattices and injected alternatingly. The solutions contain La(III)- and Mn(II)acac (LMO sublattice) respectively Sr(II)-, and Mn(II)acac (SMO sublattice). The growth process was monitored using in-situ optical ellipsometry. In a subsequent step copper (Cu) films were deposited on top of MAD-grown samples via electron beam physical vapour deposition in ultra-high vacuum (UHV) conditions. Copper deposition was monitored in-situ using a quartz balance and ex-situ via X-ray reflectometry (XRR) measurements. Structural characterization is presented in detail in the next paragraph.
\par\mekskip
Something about XRR/XRD etc
\par\mekskip
\begin{table}[ht]
	\centering
	\caption{The data of X-ray reflectivity (XRR) and X-ray diffraction (XRD) for all SLs. Individual thicknesses of layers $d_\text{SMO}$ and $d_\text{LMO}$ were obtained from simulations by using of \textit{ReMagX} program (\cite{smacke2014}) and the mean out-of-plane lattice parameters, $\text{C}_{00\text{p}}$, from the measured XRD patterns. $\text{n}_\text{exp}$ and $\text{m}_\text{exp}$ are evaluated form XRR and XRD thicknesses of SMO and LMO layers, respectively.}
	\label{fig:T_and_H}
	\begin{tabular}{|l|l|l|l|l|l|l|l|}
		\hline
		\multicolumn{2}{|l|}{(SMO$_{n}$/LMO$_{m}$)$_{10}$} & \multicolumn{2}{l|}{XRR} & \multicolumn{2}{l|}{XRD} & \multicolumn{2}{l|}{} \\ \hline
		n & m & $d_{SMO}$ {[}nm{]} & $d_{LMO}$ {[}nm{]} & $\Lambda$ {[}nm{]} & $\tilde{c}_{oop}$ {[}\si{\angstrom}{]} & n$_{exp}$ & m$_{exp}$ \\ \hline \hline
		1 & 1 & \multicolumn{2}{|c|}{0.3783} & 0.7566 & 0.3783 & \multicolumn{2}{|c|}{1.0} \\ \hline
		2 & 2 & \multicolumn{2}{|c|}{0.7580} & 1.5160  & 0.3790 & \multicolumn{2}{|c|}{2.0} \\ \hline
		3 & 3 & 1.1 & 1.1 & 2.3 & 3.82 & 2.9 & 2.9 \\ \hline
		4 & 4 & 1.5 & 1,5 & 3.0 & 3.82 & 4,0 & 3.9 \\ \hline
		5 & 5 & 1.7 & 2.0 & 3.8 & 3.82 & 4.6 & 5.3 \\ \hline
		6 & 6 & 2.0 & 2.2 & 4.2 & 3.82 & 5.5 & 5.6 \\ \hline
		%10 & 10 & 3,5 & 3,9 & 7,2 & 3,82 & 9,2 & 10,0 \\ \hline
	    \end{tabular}
\end{table}
\FloatBarrier

\appendix\subsection{\label{sup:ttr_model}Numerical model of transient thermoreflectivity}

ACHTUNG! Nur Platzhalter. Dieser Teil vom Sup wird noch neu geschrieben!!!
To extract information about the thermal conductivity of the superlattice structure, the measured TTR curves are compared to an analytic description of heat transport, as introduced by Balageas et al. \cite{Balageas1986}.
In general, thermal transport in a multilayer can be described classically by a system of coupled partial differential equations. To simplify the calculations, we assume the direction of the heat transport to be purely normal to the sample surface. The mathematical problem then reduces to a single spatial dimension. The system consists of one Fourier (diffusion) equation (Eq. \eqref{eq:diffusion}) for each material layer (namely the Cu-capping layer, the SL-layer and the STO-substrate) plus interface conduction equations between neighboring layers (Eq. \eqref{eq:boundary}), and boundary conditions at the top and bottom of the sample. As initial condition, we assume that the energy of the pump laser is absorbed at the surface of the Cu-capping layer at $z=0$ at time $t=0$ (Eq. \eqref{eq:start}).
\begin{align}
\label{eq:diffusion}
\frac{\partial T_i}{\partial t} = \frac{\kappa_i}{\rho_i c_i} \frac{\partial^2 T_i}{\partial z^2}, i\in\{1,2,3\}
\end{align}
\begin{align}
\label{eq:start}
-\kappa_1 \frac{\partial T_1}{\partial z}(z=0,t) = \delta(t)
\end{align}
\begin{multalign}
	\label{eq:boundary}
	-\kappa_i \frac{\partial T_i}{\partial z}(z_i,t) = 	-\kappa_{i+1} \frac{\partial T_{i+1}}{\partial z}(z_{i+1},t)\\ = h_i\left[T_i(z_i,t)-T_{i+1}(z_i,t)\right]
\end{multalign}
Upon applying a Laplace transform, the equations change from the time domain to the Laplace space. Thereby the time-derivatives vanish and become multiplicative expressions.
The remaining normal differential equations can be solved with an appropriate ansatz for each layer:
\begin{multalign}
	\tilde{T}_i = A_i(s)\sinh\left((z-z_{i-1})\sqrt{\frac{\rho_i c_i}{\kappa_i}s}\right)\\ + B_i(s)\cosh\left((z-z_{i-1})\sqrt{\frac{\rho_i c_i}{\kappa_i}s}\right).
\end{multalign}
Here $\tilde{T}_i$ is the Laplace-transformed temperature at the $i$-th layer and $z_{i}$ the $i$-th boundary position with $i=0$ being the surface of the sample.
The ansatz results in a system of six linear equations, $M\cdot \vec{a} = (1,0,0,0,0,0)^T$. Here, $\vec{a}$ contains the unknown constants of the ansatz ($A_i,B_i$). The system can be solved for the surface temperature in Laplace-space, which corresponds to the second entry $a_2$ of  $\vec{a}$:

\begin{align}
\tilde{T}_{surf}(s) = b_1(s) = \det(M_{12}^\downarrow)/\det(M),
\end{align}
Where $M_{12}^\downarrow$ is the minor matrix, which is obtained by omitting the first row and second column of $M$. To obtain time dependent expression, the inverse Laplace transform of $T_{surf}(s)$ is calculated. This requires solving a complex integral by means of the residual theorem:

\begin{multalign}
	T_{surf}(t) &\propto\\ 1 + \sum_{i=1}^\infty( \det(M_{12}^\downarrow)/(\partial \det(M)/\partial s) ) &\cdot exp(s_i \cdot t)
\end{multalign}
The arguments $s_i$ of the exponentials are the real, negative roots of $\det(M)$, which give rise to poles of $T_{surf}(s)$, which contribute to the inverse Laplace transform according to the residual theorem.

The final solution is an infinite series of weighted decaying exponentials, proportional to the surface temperature and therefore to the reflectivity measured in TTR. The numerically obtained curves are parametrized by the material properties of the layers, as well as by the interface conductances. Note that we truncate the series after the 2000th term. Larger summands only contribute to very small time scales $<5\,$ns directly after the excitation, where this model does not hold true anyway, because of the assumed delta peak as starting condition.

We then use non-linear optimization to best approximate the measured data with our numerical solution in the form of a least squares-fit. The free parameters are the interface conductivities between the SL and the Cu layer, and between the SL and the substrate, as well as the effective thermal conductivity of the SL. The other necessary parameters for the description of the samples are taken from literature, and are listed in table 1.

Because of our assumption that the interface conductivities do not depend on the superlattice period $m+n$, these parameters are optimized simultaneously for all samples with the same $m/n$. The optimization method of choice is the Nelder-Mead method, which is a derivative free algorithm and therefore very stable and fast. It optimizes the parameters by iteration, where in each step the values on the corners of a multidimensional simplex are compared and said simplex modified (e.g. by scaling, mirroring or stretching).

%tabelle bitte in table umgebung und anders sortieren wie besprochen

\vspace{2cm}
\begin{table}
	\captionof{table}{This table shows assumed and fitted values (including error margins) for heat capacities $c_{p,\ce{x}}$, mass densities $\rho_{\ce{x}}$, and interfacial conductances $h_{\ce{x}\leftrightarrow\ce{y}}$.}
	\begin{tabular}{| c || c | c | c  | c |}
		\hline
		& $c_p$ [\SI{}{\joule\per\kilogram\per\kelvin}]& $\kappa$ [\SI{}{\watt\per\meter\per\kelvin}] & $\rho$ [\SI{}{\kilogram\per\cubic\meter}] & $h_{\ce{x}\leftrightarrow\ce{y}}$ [\SI{}{\watt\per\meter\squared\per\kelvin}]\\\hline\hline
		Cu (50 nm) & 385& 400 & 8700& \\\hline
		SL  & 532 & & 6222& 0.091(1) ($\ce{Cu}\leftrightarrow\ce{SL}$)  \\
		$m/n=1$ & & & & 1.81(2) ($\ce{LMO}\leftrightarrow\ce{SMO}$) \\\hline
		STO (0.5 mm) & 520 & 12 & 5111 & 20(1) ($\ce{SL}\leftrightarrow\ce{STO}$)   \\\hline		
	\end{tabular}
\end{table}

For each sample, the thickness of the SL layer was calculated from the nominal composition $m$ and $n$ and the lattice constant. The effective heat capacities and densities of the SLs were interpolated between LMO and SMO, according to the actual La and Sr content for a given $m$ and $n$. 
\FloatBarrier
\subsection{Numerical model of thermal conductivity}
\label{sup:numerical_model}
\begin{figure*}
	\includegraphics[width=85mm]{Figures/Supplement/FigS1bandstructureSMO.png}
	\caption{ Acoustic phonon band structure $\omega(\mathbf k)$ according to a BK model of LaMnO$_3$ (dashed red lines) and SrMnO$_3$ (solid lines) for $\xi=20c$. The depicted sections along high symmetry directions of the Brillouin zone refer to $\Gamma=\left(0,0,0\right)$, $\mathbf{X}=\left(0,0,\nicefrac{\pi}{c}\right)$, and $\mathbf{R}=\left(\nicefrac{\pi}{a},\nicefrac{\pi}{a},\nicefrac{\pi}{c}\right)$. }\label{fig:SM1}
\end{figure*}
\FloatBarrier
In the following, we describe a model in the spirit of Simkin and Mahan \cite{Simkin.2000}. To calculate the phonon thermal conductivity, generally, we evaluate 

\begin{eqnarray}
 \kappa &=&\sum_i \int_\mathrm{1.BZ} \frac{d^3k}{(2\pi)^3}\hbar\omega_i \left\vert v_z\right\vert\xi(\mathbf{k})\frac{\partial n}{\partial T}\\
 &\approx &k_\mathrm{B} \xi\sum_i \int_\mathrm{1.BZ} \frac{d^3k}{(2\pi)^3} \left\vert v_z\right\vert,\label{Eq:SLkappa}
\end{eqnarray}
where the summation extends over all phonon branches.
Note that, for simplicity, we assume a constant phonon mean free path $\xi(\mathbf k)=\xi$, as well as a classical phonon occupation statistic $n=\frac{k_\mathrm{B}T}{\hbar\omega}$. To calculate $v_z=\frac{\partial\omega_i(\mathbf k)}{\partial k_z}$, we need to know the phonon band structure $\omega(\mathbf k)$. We notice that, since optical modes have small group velocity $v_z$, they do not contribute significantly to the thermal conductivity. Therefore, we describe the relevant acoustic phonons using a simple Born-von-Kármán (BK) model for an effective one-atomic tetragonal lattice. We adopt the in-plane lattice constant $a=0.3905 $nm adopted from the SrTiO$_3$ substrate, and the out-of-plane constant $c$ from our XRD measurements. The mass of the effective atom is given inside the LaMnO$_3$ layers by $m_\mathrm{LMO}=m_\mathrm{La}+m_\mathrm{Mn}+3m_\mathrm{O}$, and inside the SrMnO$_3$ layers by $m_\mathrm{SMO}=m_\mathrm{Sr}+m_\mathrm{Mn}+3m_\mathrm{O}$. The model includes direct and next neighbours coupling, parametrized by two spring constants $K_1$ and $K_2$. Note that, in \cite{Simkin.2000} only direct neighbour coupling is considered. Thus, there only longitudinal phonon modes are accounted for. Here, also transversal modes are included. For each effective atom identified by the index $k=1...2n$, the following equation of motion holds for the three displacement components ($i=x$, $y$, $z$) in the unit cell at $\mathbf R_{\mathbf{mno}}$:
\begin{eqnarray}
m_k \frac{d^2 u_{k,i} (\mathbf R_{\mathbf{mno}},t)}{d t^2}=-K_1\sum_{j=1...6} \hat n_{j,i}\left[\mathbf u(\mathbf R_{\mathbf{mno}},t)-\mathbf u(\mathbf R_{\mathbf{mno}}+\mathbf n_j,t)\right]\cdot\hat{\mathbf n}_j\\
-K_2\sum_{j=1...12} \hat{nn}_{j,i}\left[\mathbf u(\mathbf R_{\mathbf{mno}},t)-\mathbf u(\mathbf R_{\mathbf{mno}}+\mathbf{nn}_j,t)\right]\cdot\hat{\mathbf{nn}}_j,
\end{eqnarray}
where $\mathbf n_j$ ($\hat{\mathbf n}_j$), and $\mathbf{nn}_j$ ($\hat{\mathbf{nn}}_j$) are (normalized) vectors pointing to direct and next-neighbour atoms. With the usual ansatz of plane waves, one can obtain the phonon spectrum $\omega(\mathbf k)$ by solving the eigenvalue problem 
\begin{equation}
	\mathbf M\cdot \mathbf e=-\omega^2 \mathbf e, 
\end{equation}
where the entries of system matrix $\mathbf M$ are functions of the complex wave numbers $k_i+\nicefrac{\imath}{\xi}$ ($i=x,\,y,\,z$). The numerical values for the spring constants are chosen such that we get typical longitudinal and transverse sound velocities ($v_\mathrm{l}=6500\,$m/s, $v_\mathrm{t}=3500\,$m/s) for cubic SrMnO$_3$. Figure \ref{fig:SM1} shows the acoustic phonon spectra of pure SMO and LMO as a computed with our BK model. Note that, cubic LaMnO$_3$ is actually not stable as an isolated crystal at room temperature, where the oxygen octahedra are normally rotated. Only inside our SLs with $m=n$ a cubic structure is stabilized (see \cite{V.Roddatis}). As simple assumptions, we here take the same force constants $K_1$ and $K_2$ for both SrMnO$3$, and LaMnO$_3$, and only vary the masses of the effective atoms as introduced above.

\begin{figure*}
	\includegraphics[width=160mm]{Figures/Supplement/FigS2bandstructures.png}
	\caption{ Acoustic phonon band structure $\omega(\mathbf k)$ according to a BK model of LMO/SMO SLs with $\Lambda=2n$. Different panels refer to different $n=1\,...6$ as indicated. Solid lines [dashed lines] are results obtained for a phonon mean free path of $\xi=20c$ [$\xi=5c$]. The depicted sections along high symmetry directions of the Brillouin zone refer to $\Gamma=\left(0,0,0\right)$, $\mathbf{X}=\left(0,0,\nicefrac{\pi}{\Lambda}\right)$, and $\mathbf{R}=\left(\nicefrac{\pi}{a},\nicefrac{\pi}{a},\nicefrac{\pi}{\Lambda}\right)$. }
	\label{fig:SM2}
\end{figure*}

Figure \ref{fig:SM2} shows acoustic phonon spectra for SLs, calculated assuming different value for $n$ and $\xi$ as indicated. Note that, SLs have a strongly reduced Brillouin zone along the z-direction, caused by the artificial backfolding of the bands. Before we compute the dependence of $\kappa$ on $\Lambda=2n$, we first estimate the phonon mean free path $\xi$ from the volume contribution to the thermal resistivity $\frac{1}{\kappa_v}$. According to Eq. \eqref{Eq:kappaeff}, for $\Lambda\rightarrow \infty$, the contribution from interfaces vanishes. The effective resistivity is then 

\begin{equation}
\frac{1}{\kappa_v}=\frac{1}{2\kappa_{\mathrm{LMO}}}+\frac{1}{2\kappa_{\mathrm{SMO}}}.
\end{equation}

From our previous publication \cite{V.Roddatis}, we know that $\frac{1}{\kappa_v}=0.20(1)\,$mK/W. Our model reproduces this value when assuming a phonon mean free path of $\xi_v=45c$.

\begin{figure}
	\includegraphics[width=85mm]{Figures/Supplement/FigS3conductivity.png}
	\caption{Comparison of modeling results and experimental data. Violet rectangular dots show $\kappa(\Lambda)$ for $\xi=45c$ calculated using the BK model and Eq. \eqref{Eq:SLkappa}. Oliv dots refer BK model plus Kapitza resistance due to roughness, according to Eq. \eqref{Eq:kappaeff}. Open circular dots show experimental data. Dashed horizontal line indicates the volume limit $\kappa_v=5\,$W/mK approached for $n\rightarrow \infty$. Solid lines as guides to the eye.}\label{fig:SM3}
\end{figure}

Evaluating Eq. \eqref{Eq:SLkappa} as a function of the SL period $\Lambda$ for $\xi=\xi_v$ yields the data shown in Fig. \ref{fig:SM3}. One sees a minimum of $\kappa$ at $\Lambda=6a_z$.  Compared to \cite{Simkin.2000}, the minimum is rather shallow. Comparing the maximum at $\Lambda=2$ with the minumum at $\Lambda=6$, one sees a reduction of about $22\%$.

Note that, the conductivities are for finite $n$, and $\xi=\xi_v$ generally much larger than the experimentally found conductivities. The reason is that, in our model, the Kapitza resistance is underestimated, because interface roughness is not taken into account. The phonon mean free path entering the calculation parametrizes dissipation effects inside the volume of the bilayers. To include roughness, one can add after the calculation the missing interface contribution according to Eq. \eqref{Eq:kappaeff}. Better agreement with experimental data can be obtained with an interfacial resistivity of $h=2.7$ GW/m$^2$K, as the oliv data points shown Figure \ref{fig:SM2} demonstrate. But also then, for $\Lambda <6$ the model still deviates from the experimental data. In the main article we follow a different approach. Instead of adding additional interface contributions afterwards, there we adjust $\xi$ as a free parameter for each sample.

\appendix\subsection{Matching of $\kappa$ and $\xi$}
\label{sup:matching}
\begin{figure*}
	\centering
\includegraphics[width=80mm]{Figures/resultswithmfp.png}
\caption{Numerical model for different MFP $\xi$ and the measurements of $\kappa$ from the TTR experiment (white circles).\label{fig:matching}}
\end{figure*}
For the extraction of the phonon mean free path from our TTR measurements we evaluated the numerical model for different MFP and matched the $\kappa$ values obtained from fitting the reflectivity measurements to thease curves, pactically projecting each $\kappa$ to a $\xi$.
